# Supplementary material for: Phenomenology of the minimal $B-L$ Model: the Higgs sector at the Large Hadron Collider and future Linear Colliders
Source: arXiv:1106.4691 source file (2011-06-23)
Supplement: Supplementary file 1 [file AppendixD.tex]

\chapter{The $e^+e^- \rightarrow h_1 h_1$ cross-section}
\label{appe:d}
\lhead{Appendix D. \emph{The $e^+e^- \rightarrow h_1 h_1$ cross-section}}

The leading order contribution to the process $e^+e^-\rightarrow
h_1h_1$ is the one related to the one-loop box diagrams in figure
\ref{boxeeh1h1} (and their crossed diagrams).

\begin{figure}[!ht]
  \subfigure[]{
  \label{boxee-w-h1h1}
  \includegraphics[angle=0,width=0.32\textwidth]{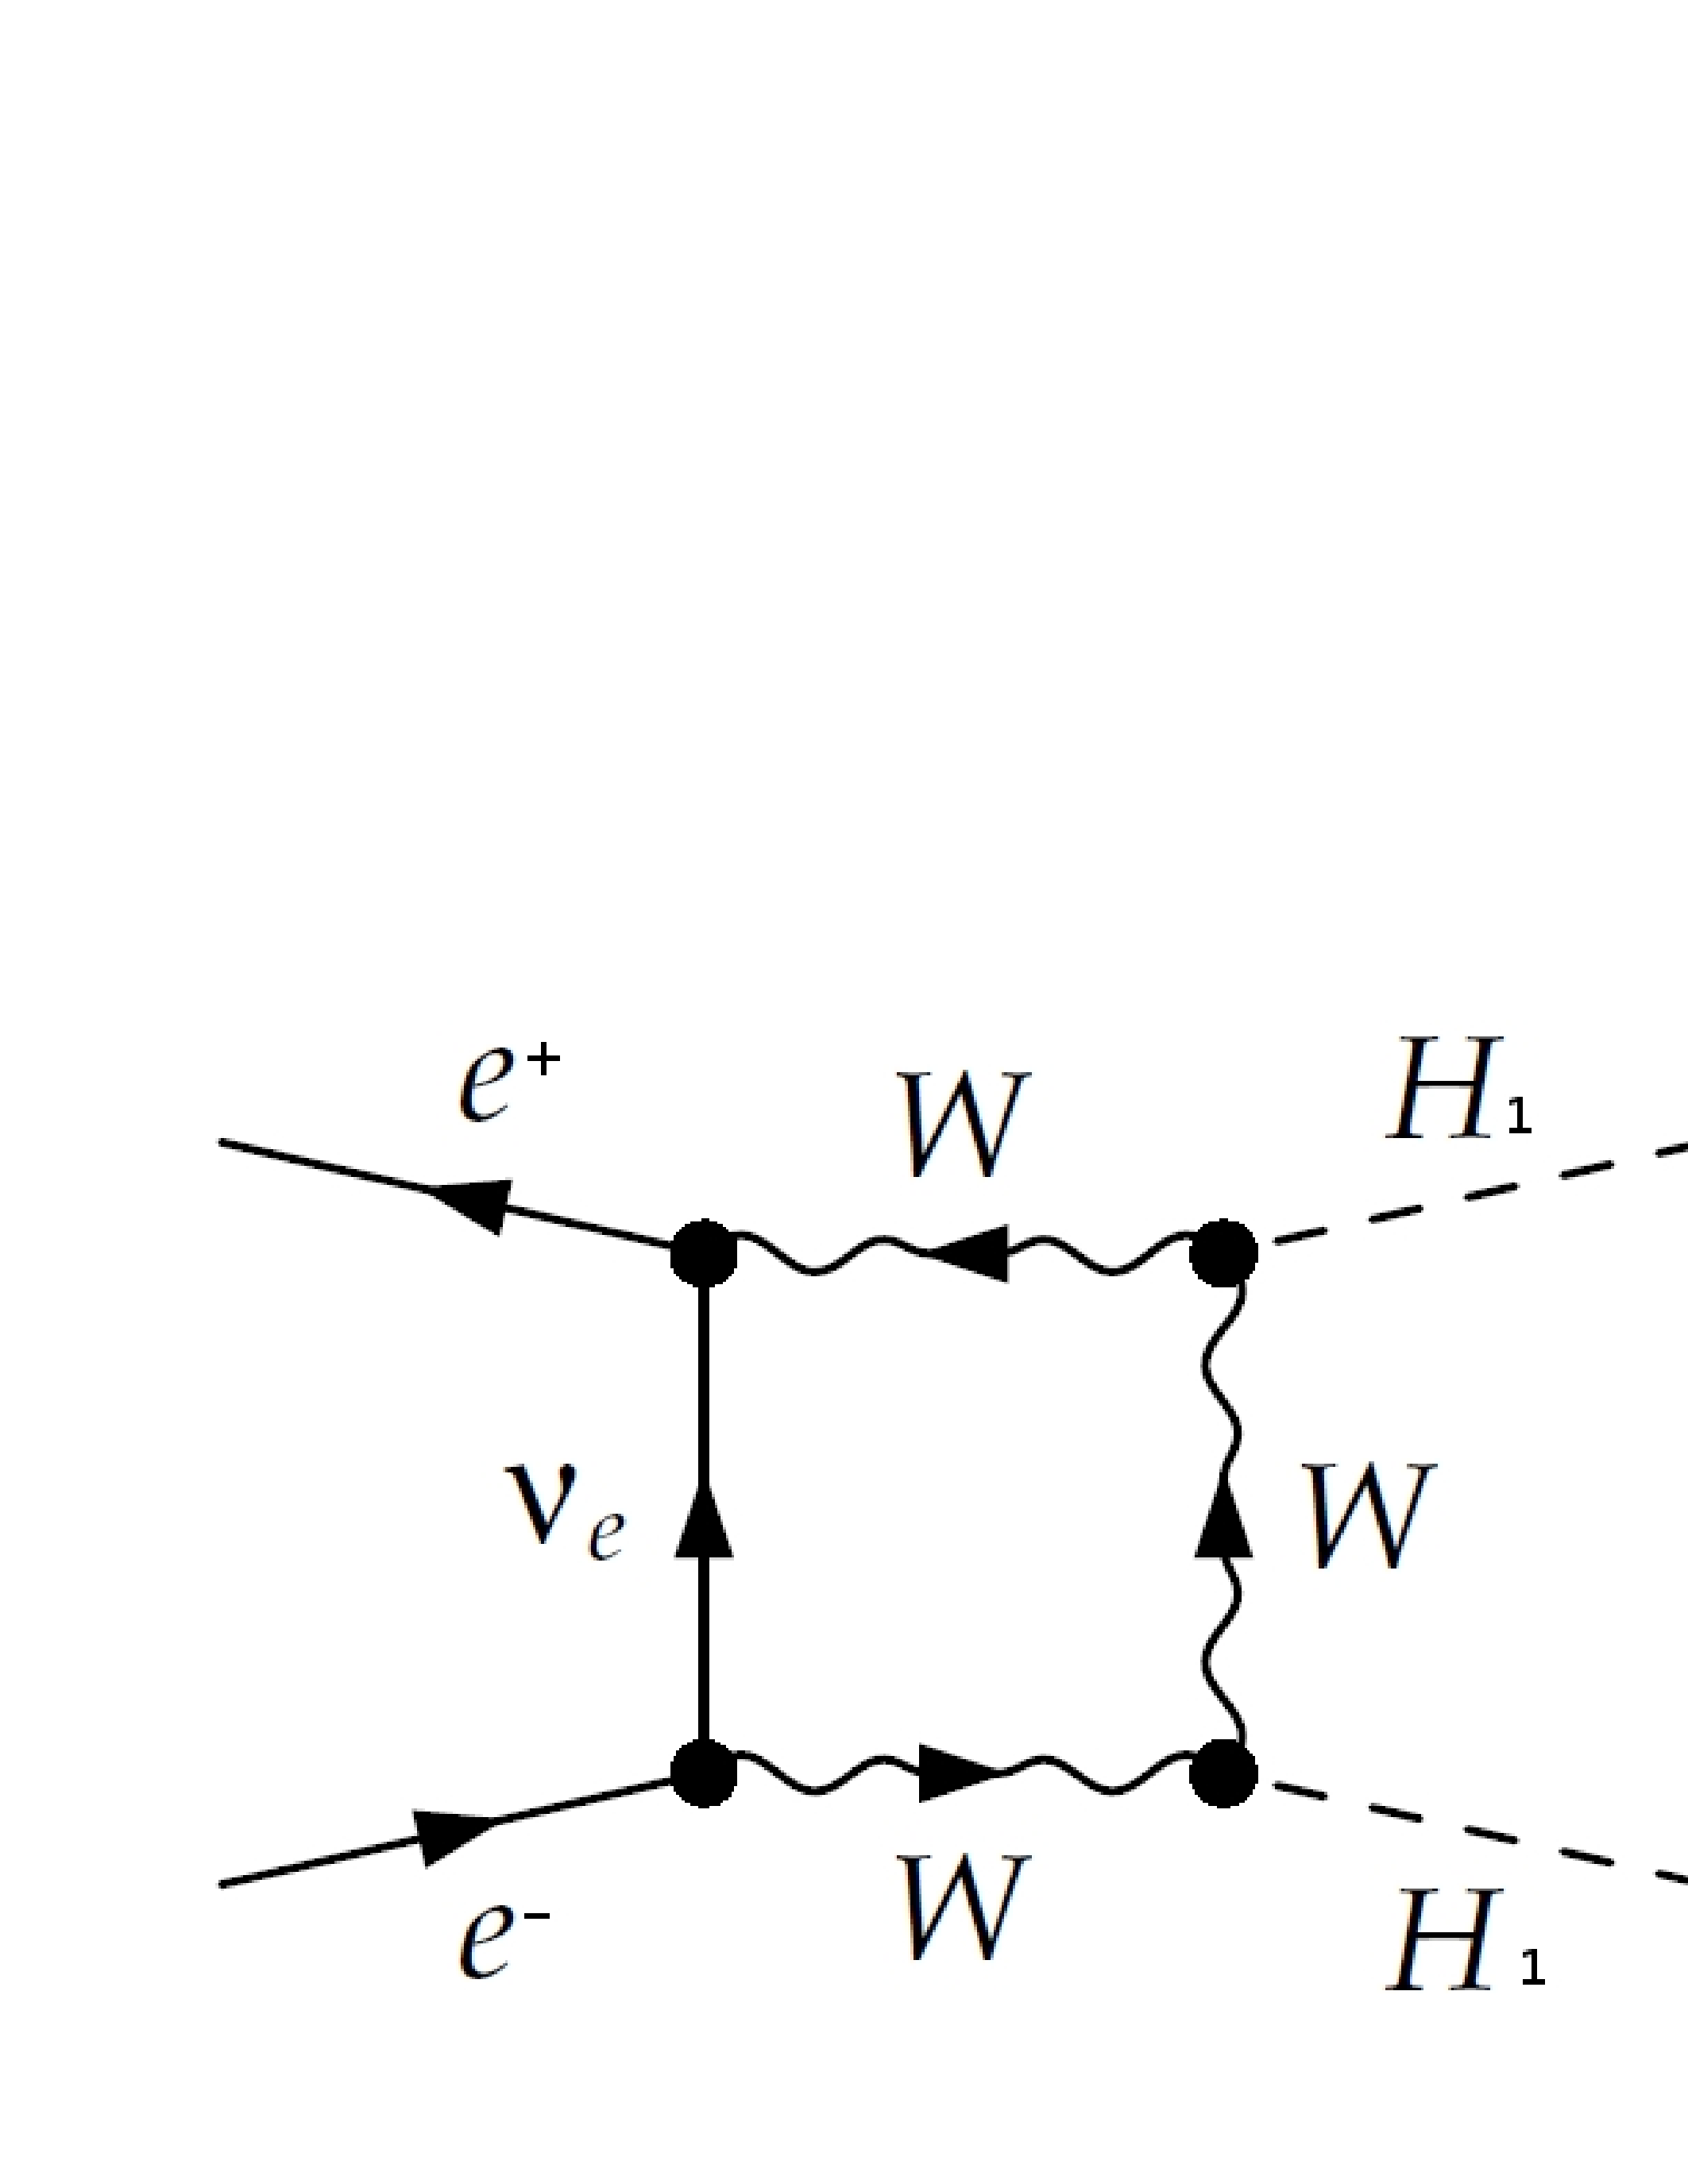}}
  \subfigure[]{
  \label{boxee-z-h1h1}
  \includegraphics[angle=0,width=0.32\textwidth]{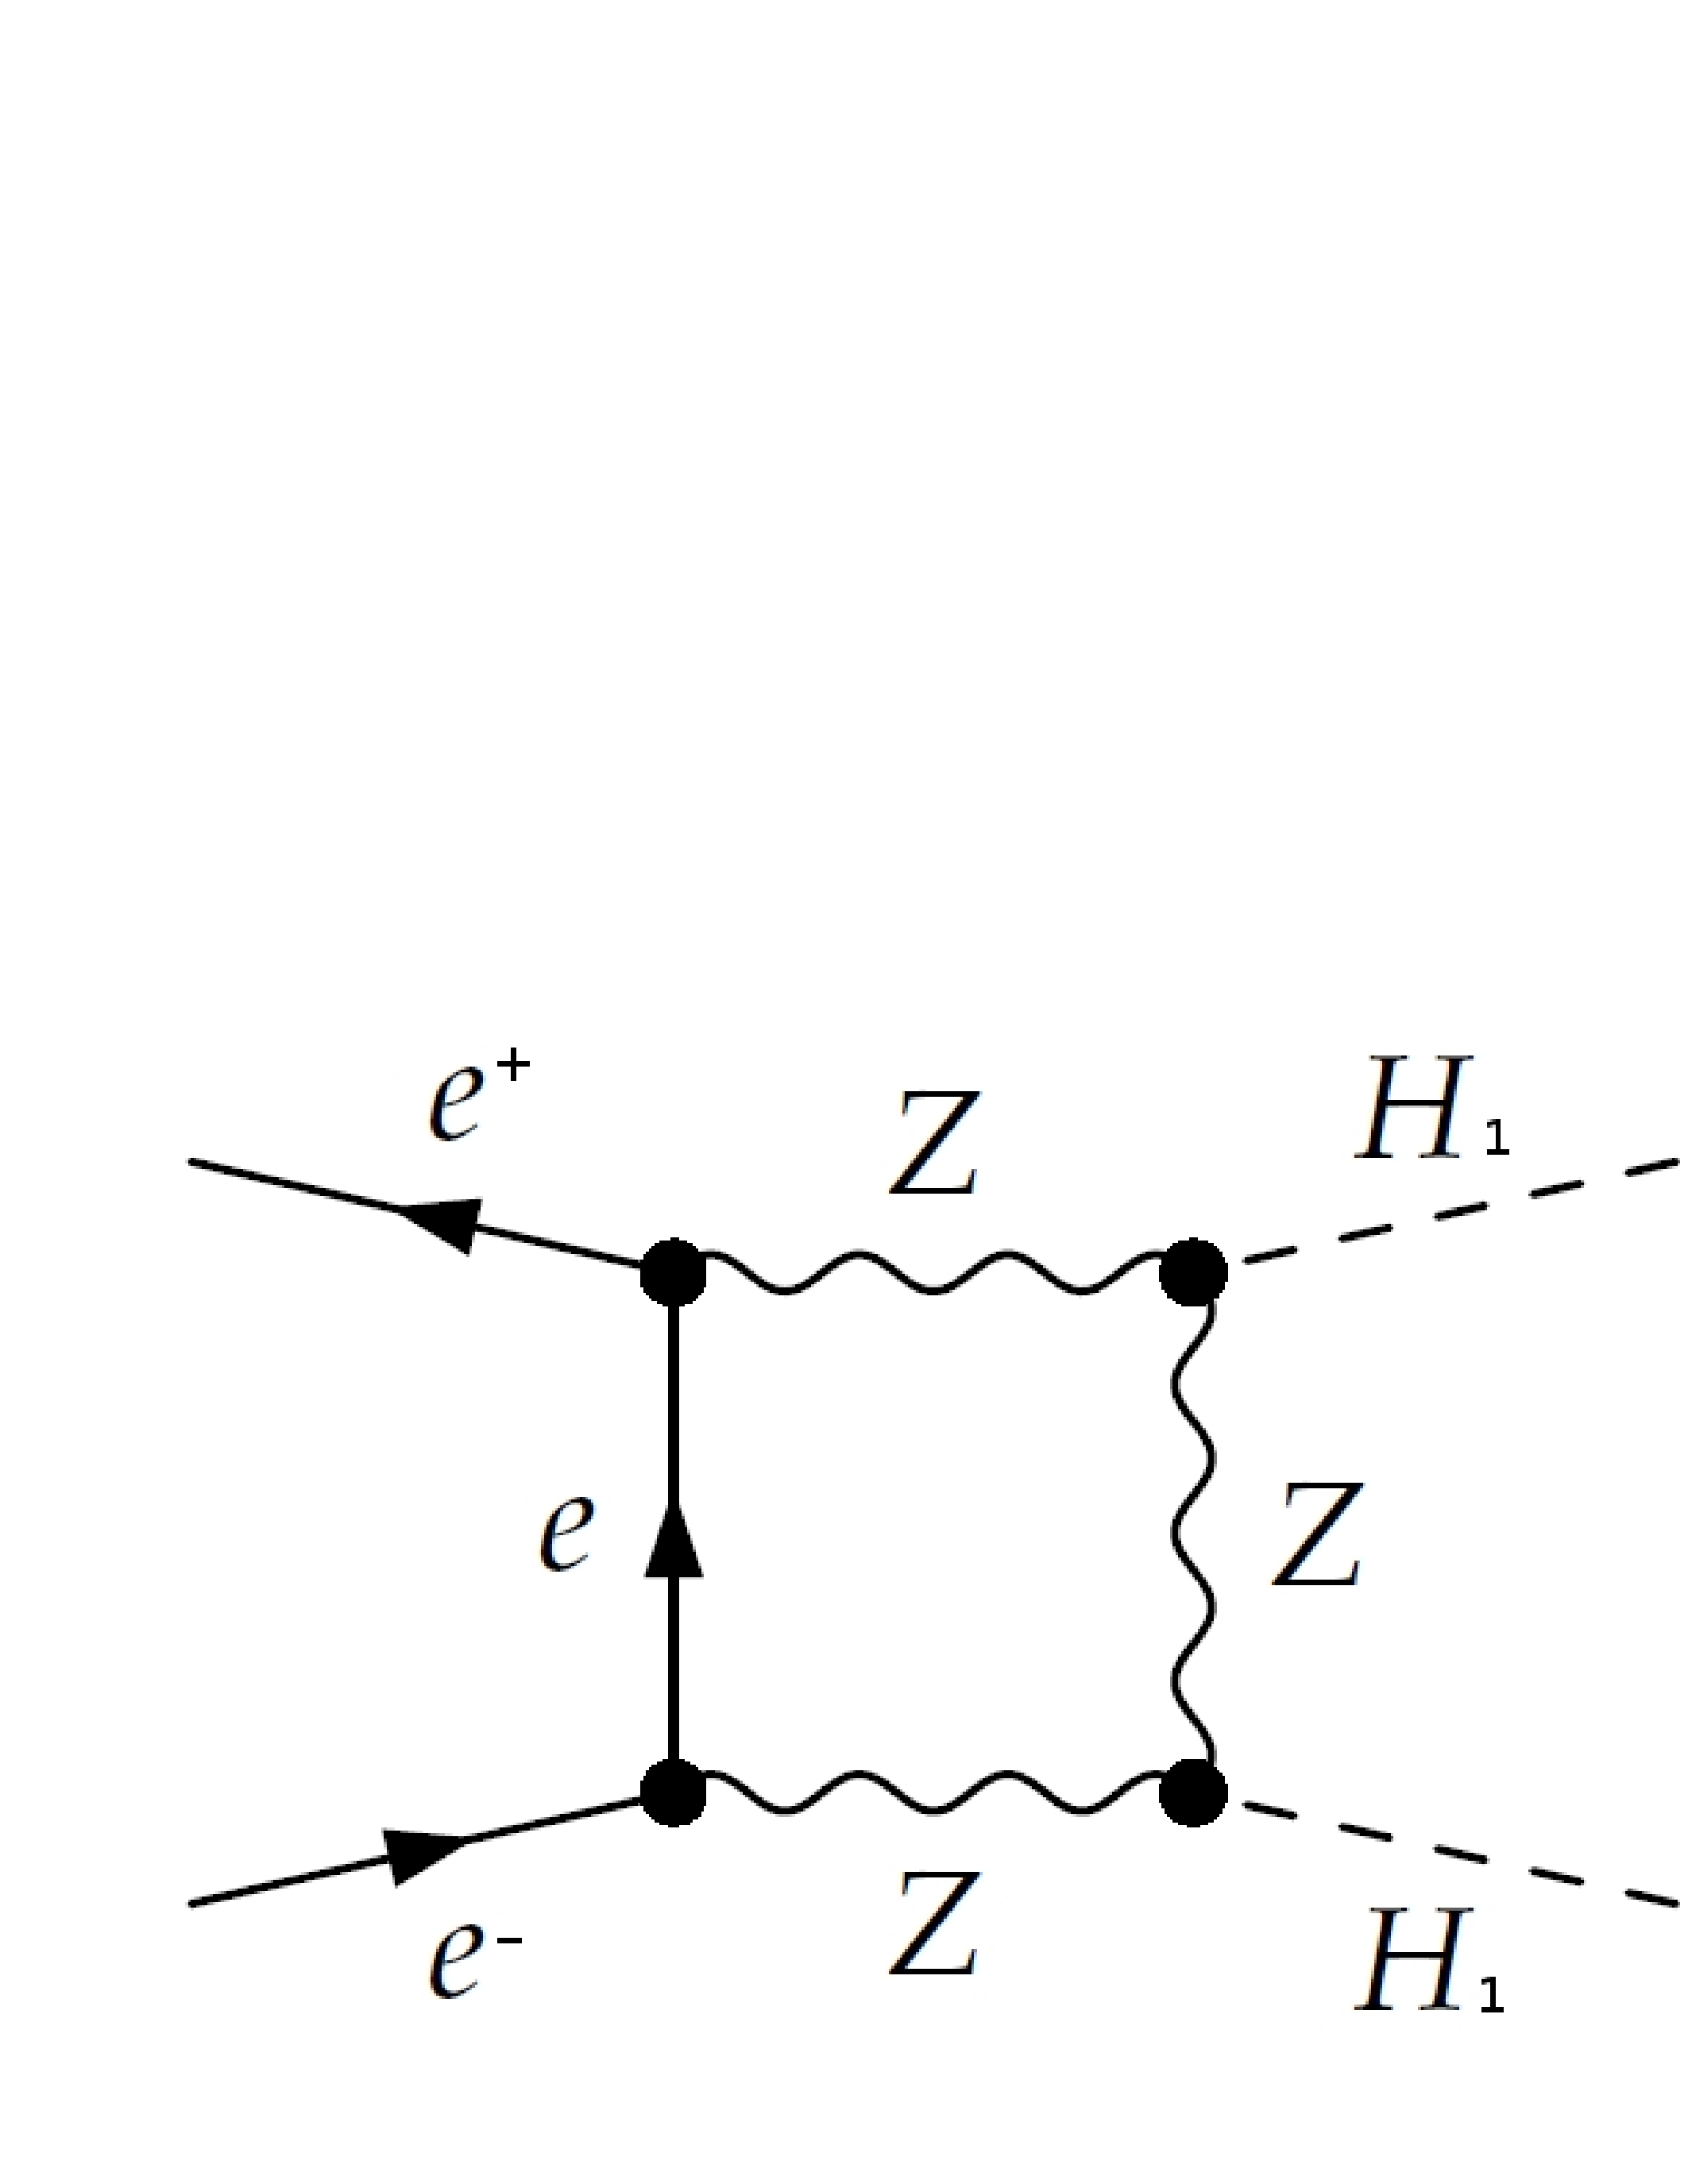}}
  \subfigure[]{
  \label{boxee-zp-h1h1}
  \includegraphics[angle=0,width=0.32\textwidth]{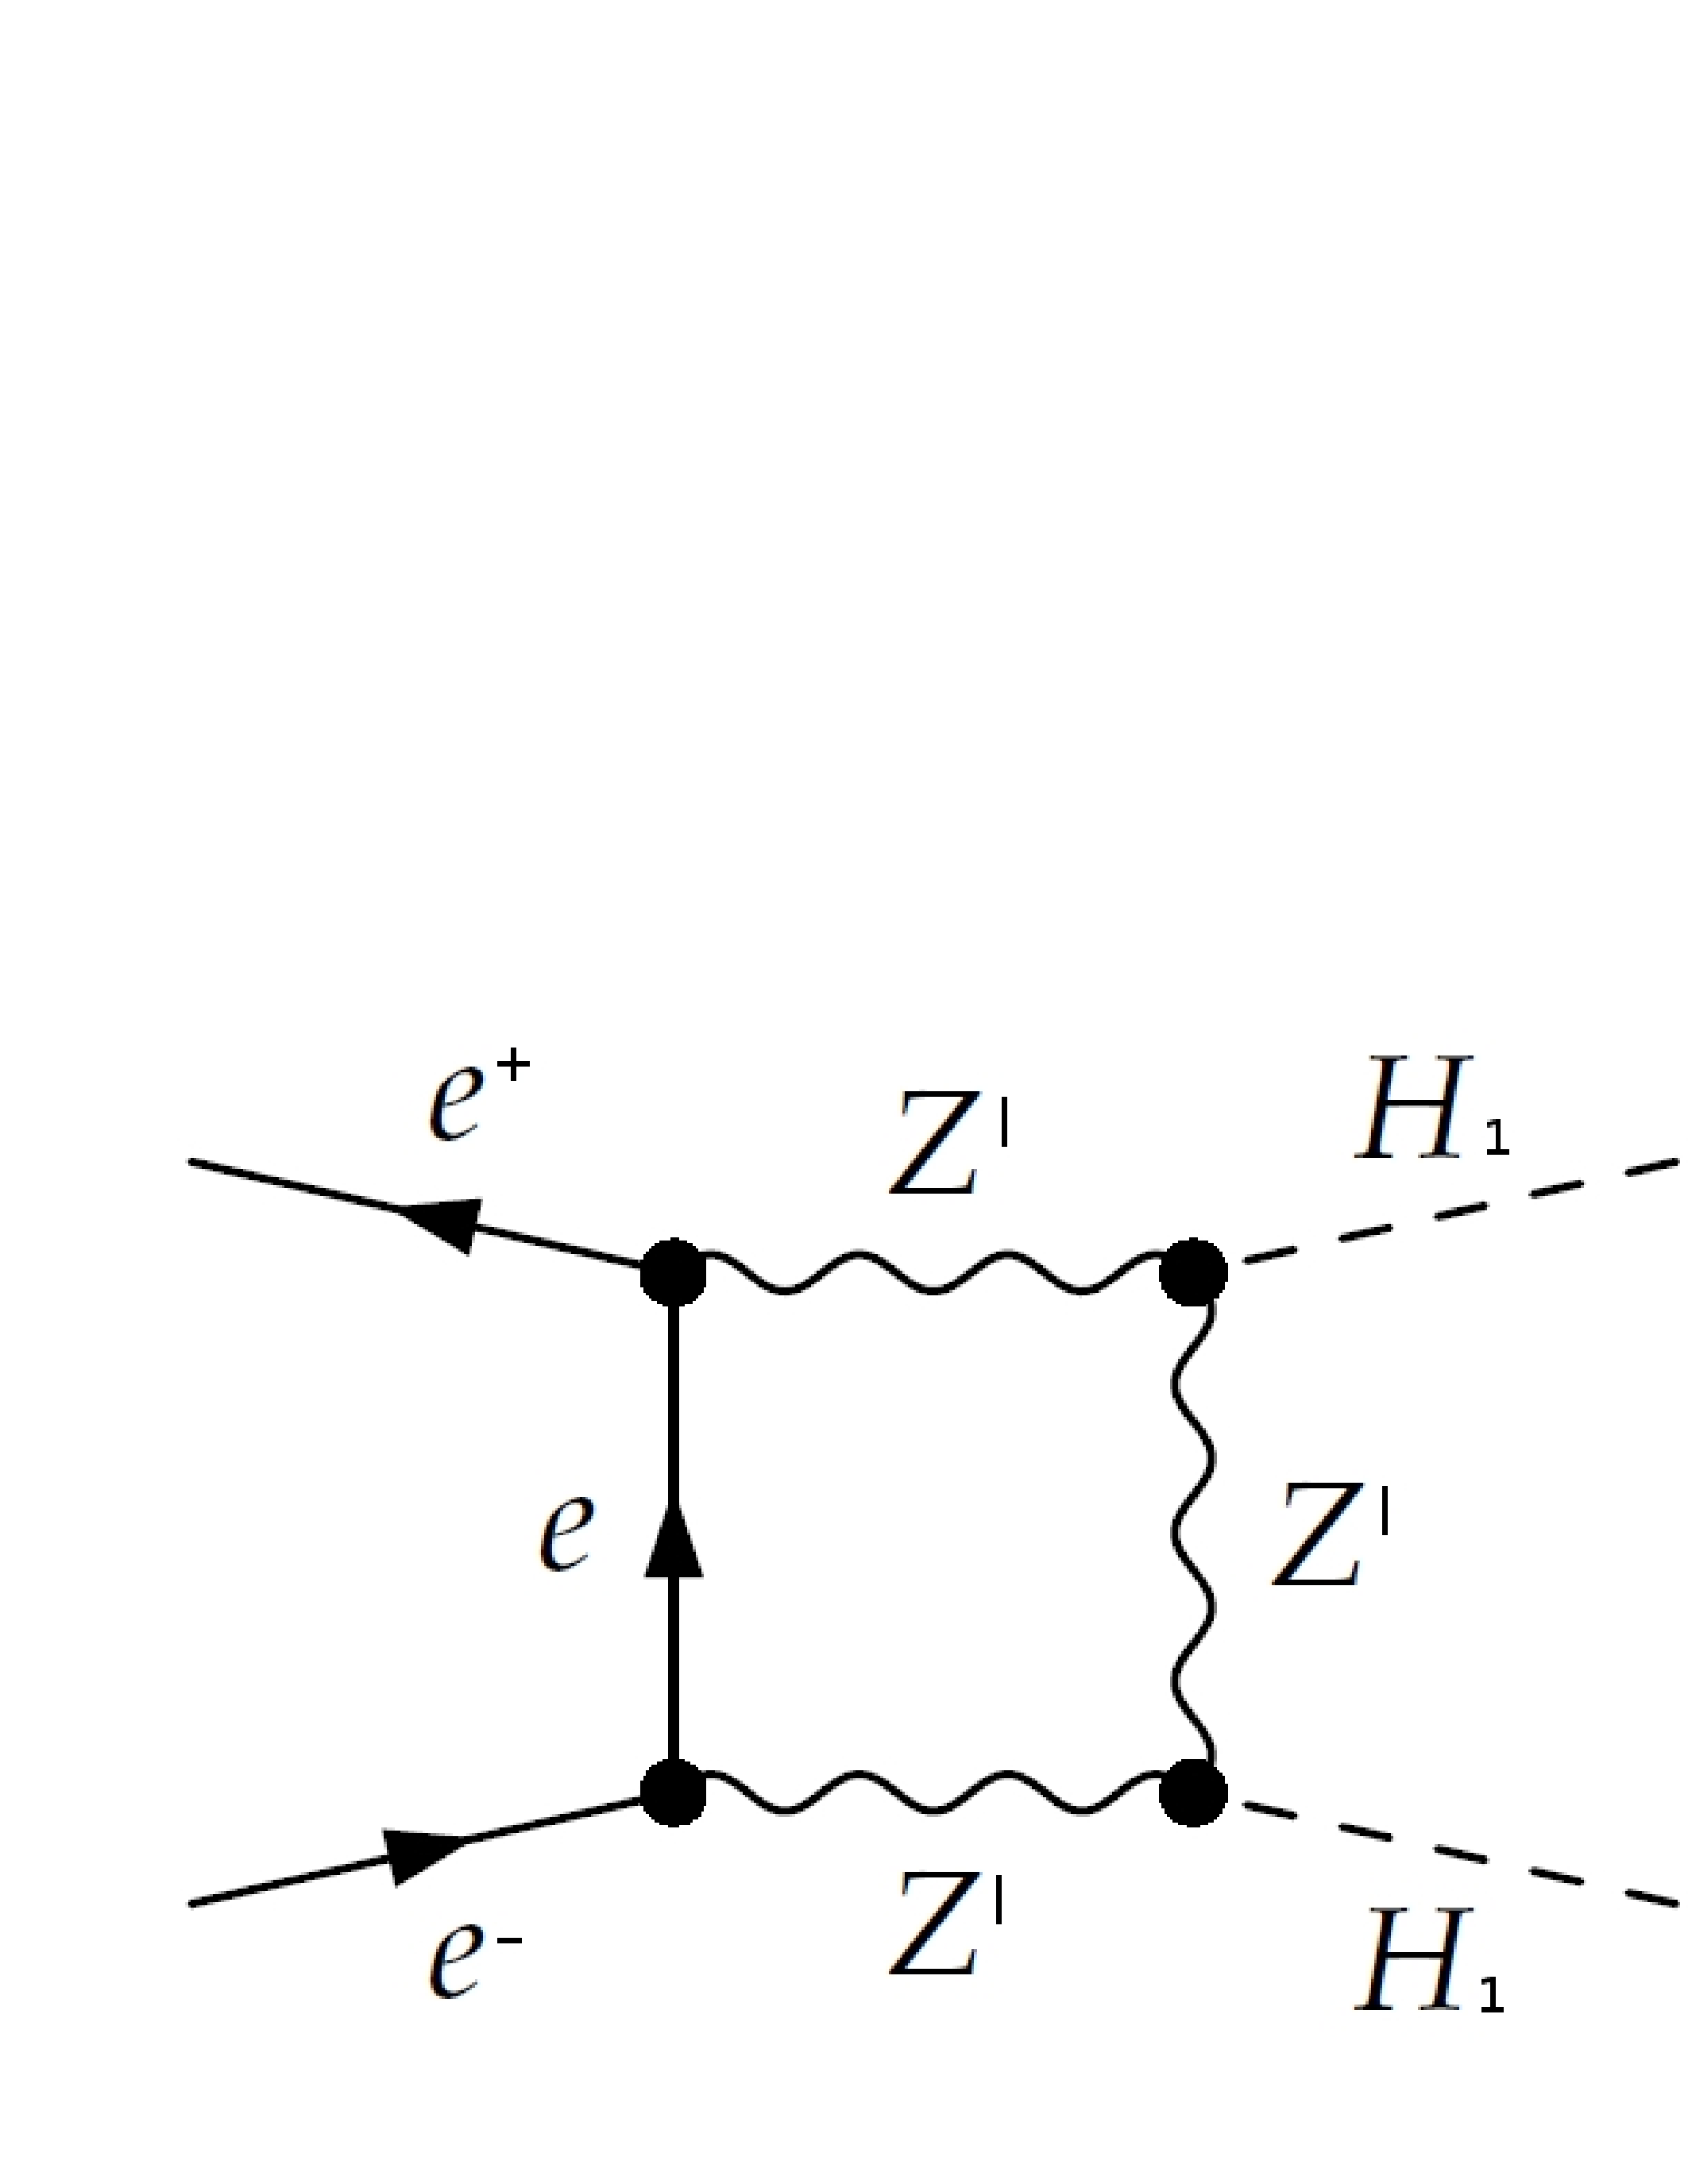}}
%  \vspace*{-0.5cm}
  \caption{Leading order contribution to $e^+e^-\rightarrow h_1h_1$ in
  the minimal $B-L$ model}
  \label{boxeeh1h1}
\end{figure}

Apart from the well known $SM$-like contributions, the only peculiar
$B-L$ ``signal'' is reprented by the diagram in figure
\ref{boxee-zp-h1h1} (and its crossed diagram).

Following the steps well-described in \cite{Gaemers:1984vw}, is
possible to obtain the helicity-dependent amplitude:

\begin{eqnarray}
\mathcal{M}_{\lambda_1,\lambda_2} &=& (\lambda_1-\lambda_2) \frac{(g_1')^4
  \sin^2{a}}{16 \pi^2} \sqrt{s^2-4M_{h_1}^2 s-u^2} \times \nonumber \\
&\times &
\left(4 C_0 + C_{2} - M_{h_1}^2 D_{22} + 4 M_{h_1}^2 D_{3}
+ 4 M_{Z'}^2 D_{0} + s D_{12} + s D_{22} - 2 s D_{3} + \right. \nonumber \\
&+& \left. \left(4 M_{h_1}^2 + 9 M_{Z'}^2 + s \right) D_2 + 2 
\left(2 M_{h_1}^2 + s - 2 u \right) D_1 + u D_{22} - 4 u D_{3} \right),
\end{eqnarray}
where the $C$'s and $D$'s are the well-known Passarino-Veltman
functions (we assume the convention of \cite{Denner:1991kt,Hahn:1998yk}):
\begin{eqnarray}
&\ &C_i(0,M_{h_1}^2,t,0,M_{Z'}^2,M_{Z'}^2), \nonumber \\
&\ &D_i(0,M_{h_1}^2,M_{h_1}^2,0,t,s,0,M_{Z'}^2,M_{Z'}^2,M_{Z'}^2).
\end{eqnarray}

The crossed diagram is obtained by the transformation $t
\longleftrightarrow u$ in the Passarino-Veltman structure.

The cross-section is then given by the well-known formula:

\begin{equation}
\frac{d\sigma_{\lambda_1,\lambda_2}}{d\Omega}=
\frac{1}{64\pi^2s}\frac{|\mathcal{M}_{\lambda_1,\lambda_2}|^2}{2}
\sqrt{1-\frac{4M_{h_1}}{s}}.
\end{equation}
