# Supplementary material for: Phenomenology of the minimal $B-L$ Model: the Higgs sector at the Large Hadron Collider and future Linear Colliders
Source: arXiv:1106.4691 source file (2011-06-23)
Supplement: Supplementary file 2 [file AppendixC.tex]

\chapter{The Veltman solution}
\label{appe:c}
\lhead{Appendix C. \emph{The Veltman solution}}

\begin{eqnarray}
&\ & m_{h_1}^2 \simeq \nonumber \\
&\simeq &\left(3 \left((g_1') m_{Z'} v \left(12 
c_a^4 m_{\nu h}^2-8 m_t^2+4 m_W^2+2 m_Z^2-3 
m_{Z'}^2-16 c_a^2 s_a^2 v^2 (y^\nu)^2\right)+ \right. \right. \nonumber \\
&+& \left. \left. (g_1') 
m_{Z'} v \left(-12 c_a^4 m_{\nu h}^2-8 m_t^2+4 
m_W^2+2 m_Z^2+3 m_{Z'}^2-16 c_a^2 s_a^2 
v^2 (y^\nu)^2\right) \cos{(2 \alpha)}+\right. \right. \nonumber \\
&+& \left. \left. 8 c_a^4 (g_1')^2 
m_{\nu h}^2 v^2 \sin{(2 \alpha)}+m_{Z'}^2 \left(-4 m_t^2+2 
m_W^2+m_Z^2-2 (g_1')^2 v^2\right) \sin{(2 \alpha)}-\right. \right. \nonumber \\
&-&\left. \left. 8 
c_a^2 m_{Z'}^2 s_a^2 v^2 (y^\nu)^2 \sin{(2
  \alpha)}- 4 
\sqrt{2} c_a^3 m_{\nu h} s_a v (y^\nu) \left(2 \cos{(\alpha)} 
\sec{(2 \alpha)} \sin{(\alpha)} \times
\right. \right. \right. \nonumber \\ 
&\times &\left. \left. \left. \left(8 (g_1')^2 v^2 
\cos^2{(\alpha)}+3 m_{Z'}^2
\sin^2{(\alpha)}\right)+ 3(g_1') 
m_{Z'} v \sin{(2 \alpha)} \tan{(2 
  \alpha)}\right)\right)\right)\div \nonumber \\
&\div & \left(-12 (g_1') m_{Z'} v 
\cos{(2 \alpha)}+\left(-3 m_{Z'}^2+4 (g_1')^2 v^2\right) 
\sin{(2 \alpha)}\right).
\end{eqnarray}

\begin{eqnarray}
&\ &m_{h_2}^2 \simeq \nonumber \\
&\simeq &\left(3 \left((g_1') m_{Z'} v \left(-12
c_a^4 m_{\nu h}^2+8 m_t^2-4 m_W^2-2 m_Z^2+3
m_{Z'}^2+16 c_a^2 s_a^2 v^2 (y^\nu)^2\right)+ \right. \right. \nonumber \\
&+&\left. \left. (g_1')
m_{Z'} v \left(-12 c_a^4 m_{\nu h}^2-8 m_t^2+4
m_W^2+2 m_Z^2+3 m_{Z'}^2-16 c_a^2 s_a^2
v^2 (y^\nu)^2\right) \cos{(2 \alpha)}+\right. \right. \nonumber \\
&+&8 \left. \left. c_a^4 (g_1')^2
m_{\nu h}^2 v^2 \sin{(2 \alpha)}+m_{Z'}^2 \left(-4 m_t^2+2
m_W^2+m_Z^2-2 (g_1')^2 v^2\right) \sin{(2 \alpha)}- \right. \right. \nonumber \\
&-&\left. \left. 8
c_a^2 m_{Z'}^2 s_a^2 v^2 (y^\nu)^2 \sin{(2 \alpha)}+4
\sqrt{2} c_a^3 m_{\nu h} s_a v (y^\nu) \left(2 \cos{(\alpha)}
\sec{(2 \alpha)} \sin{(\alpha)} \times \right. \right. \right. \nonumber \\
&\times &\left. \left. \left. \left(3 m_{Z'}^2 \cos^2{(\alpha)}+8
(g_1')^2 v^2 \sin^2{(\alpha)}\right)-3 (g_1') m_{Z'} v
\sin{(2 \alpha)} \tan{(2 \alpha)}\right)\right)\right) \div \nonumber
\\
&\div &\left(-12
(g_1') m_{Z'} v \cos{(2 \alpha)}+\left(-3 m_{Z'}^2+4
(g_1')^2 v^2\right) \sin{(2 \alpha)}\right).
\end{eqnarray}
